# Supplementary material for: Efficient Backpropagation with Variance-Controlled Adaptive Sampling
Source: arXiv:2402.17227 source file (2024-02-27)
Supplement: Supplementary file 1 [file appendix-trash.tex]

\section{Activation sampling}

Following the notation of \citet{katharopoulos2018not}, let's construct a MLP with $L$ layers and use $\theta_t^l\in \mathbb R^{C_{l}\times C_{l-1}}$ to denote the parameter of the $l$-th layer. Then for the $i$-th input $x^0=x_i\in \mathbb R^{1\times C_{0}}$ at time $t$, we have:
\begin{align}
    z_i^l&=x_i^{l-1}(\theta_t^l)^\top\quad l=1,\cdots,L \\
    x_i^l&=\sigma^l(z_i^l)\quad l=1,\cdots,L
\end{align}
After

% 对于层数为$L$的多层感知机，其含有$L$个线性层与$L$个激活函数交替连接。记层数为$l$的线性层权重为$\theta_t^l\in \mathbb R^{C_{l}\times C_{l-1}}$，层数为$l$的激活函数为$\sigma^l$，则对于$t$时刻的第$i$个数据输入$x^0=x_i\in \mathbb R^{1\times C_{0}}$，我们有：
% \begin{align
}
%     z_i^l&=x_i^{l-1}(\theta_t^l)^\top\quad l=1,\cdots,L \\
%     x_i^l&=\sigma^l(z_i^l)\quad l=1,\cdots,L
% \end{align}

% 由此我们得到了输出$\psi_{\theta_t}(x_i)=x_i^L$，其中$\theta_t=vectorize(\theta_t^1,\cdots,\theta_t^L)$，即为全部线性层权重的向量化表示。
